# Supplementary material for: Graph Attention Networks with Positional Embeddings
Source: arXiv:2105.04037 source file (2021-10-24)
Supplement: Supplementary file 1 [file supple.tex]

\begin{tabular}{llll}
\toprule
{} &            Cora &        Citeseer &          Pubmed \\
model          &                 &                 &                 \\
\midrule
GeomGCN-g-I    &  85.81\% (1.50\%) &  80.05\% (1.59\%) &  92.56\% (0.33\%) \\
GeomGCN-g-P    &  86.48\% (1.49\%) &  75.74\% (1.58\%) &  88.49\% (0.56\%) \\
GeomGCN-g-S    &  86.50\% (1.43\%) &  75.91\% (2.26\%) &  88.55\% (0.53\%) \\
GAT-POS-C-GS   &  87.31\% (1.40\%) &  74.71\% (1.33\%) &  85.11\% (2.57\%) \\
GAT-POS-C-PI   &  87.29\% (1.52\%) &  74.67\% (1.31\%) &  85.10\% (2.57\%) \\
GAT-POS-C-PT   &  86.61\% (1.13\%) &  73.81\% (1.27\%) &  85.09\% (2.57\%) \\
GAT-POS-T-GS   &  87.90\% (0.97\%) &  75.30\% (1.10\%) &  86.57\% (1.73\%) \\
GAT-POS-T-PI   &  85.90\% (1.47\%) &  72.88\% (1.98\%) &  85.70\% (0.94\%) \\
GAT-POS-T-PT   &  82.32\% (1.75\%) &  66.68\% (2.01\%) &  83.73\% (1.21\%) \\
GAT-POS-CG-GS  &  87.01\% (1.64\%) &  74.70\% (1.31\%) &  85.12\% (2.56\%) \\
GAT-POS-CML-PI &  87.60\% (1.69\%) &  74.77\% (1.34\%) &  85.09\% (2.59\%) \\
GAT-POS-CML-PT &  86.25\% (1.29\%) &  74.65\% (2.01\%) &  85.50\% (2.14\%) \\
\bottomrule
\end{tabular}

\begin{tabular}{llll}
\toprule
{} &       Chameleon &        Squirrel &           Actor \\
model          &                 &                 &                 \\
\midrule
GeomGCN-g-I    &  61.97\% (2.01\%) &  39.91\% (1.77\%) &  32.98\% (0.78\%) \\
GeomGCN-g-P    &  60.31\% (2.07\%) &  37.14\% (1.19\%) &  31.60\% (1.06\%) \\
GeomGCN-g-S    &  63.86\% (1.78\%) &  42.73\% (2.16\%) &  31.96\% (1.97\%) \\
GAT-POS-C-GS   &  64.39\% (2.16\%) &  43.56\% (3.15\%) &  34.78\% (1.00\%) \\
GAT-POS-C-PI   &  67.65\% (2.82\%) &  42.58\% (1.66\%) &  34.65\% (1.21\%) \\
GAT-POS-C-PT   &  67.76\% (2.54\%) &  52.90\% (1.55\%) &  34.89\% (1.38\%) \\
GAT-POS-T-GS   &  65.99\% (2.66\%) &  47.79\% (2.16\%) &  34.75\% (1.16\%) \\
GAT-POS-T-PI   &  63.79\% (2.35\%) &  47.96\% (3.29\%) &  34.59\% (1.01\%) \\
GAT-POS-T-PT   &  65.55\% (2.38\%) &  51.62\% (1.84\%) &  31.97\% (1.27\%) \\
GAT-POS-CG-GS  &  65.92\% (2.29\%) &  48.39\% (1.61\%) &  34.89\% (1.08\%) \\
GAT-POS-CML-PI &  66.67\% (2.15\%) &  47.44\% (2.33\%) &  34.98\% (1.04\%) \\
GAT-POS-CML-PT &  67.48\% (3.08\%) &  50.94\% (2.77\%) &  35.03\% (1.44\%) \\
\bottomrule
\end{tabular}
